# Supplementary material for: Two-photon pumped lead halide perovskite nanowire lasers
Source: arXiv:1510.03987 source file (2015-10-14)
Supplement: Supplementary file 1 [file supplemental_information.pdf]

# Supplementary information for: Two-photon pumped lead halide perovskite nanowire lasers

Zhiyuan Gu[1, ‡], Kaiyang Wang[1, ‡], Wenzhao Sun[1], Jiankai Li[1], Shuai Liu[1], Qinghai Song[1, *], Shumin Xiao[2, †]

1. Integrated Nanoscience Lab, School of Electrical and Information Engineering, Harbin Institute of Technology, Shenzhen, China, 518055

2. Integrated Nanoscience Lab, School of Material Science and Engineering, Harbin Institute of Technology, Shenzhen, China, 518055

‡ These authors contribute equally to this research.

† shuminxiao@gmail.com

* qinghai.song@hitsz.edu.cn

In the main text, we have studied the two-photon pumped perovskite nanowire lasers. In this supplementary information, we show the details of scanning electron microscope (SEM) images of perovskite nanowires to count the length and width of perovskite nanowires. We also show the two-photon photoluminescence and lasing behaviors of different perovskite nanowire to show the generality of two-photon pumping nanolasers.

## 1. Top-view of SEM images of perovskite nanowire

After the synthesis of the perovskite nanowires, we have characterized their lengths and widths with SEM images. In Fig. S1(a), we show the SEM images 32 nanowires on the same wafer. Several characteristics can be observed. (i) There are always some rectangle shaped microdisks around the nanowires. And their sizes are quite different. (ii) While the sizes of nanowires also vary, their exact values are very close and fall in particular regions. The latter one

can be more clearly seen in Figs. S1(b) and S1(c), where the statistics of nanowire sizes are shown. We can see that most of nanowires have the lengths between 12.5 μm – 25 μm. Meanwhile, their widths are primarily around 500 nm – 1250 nm.

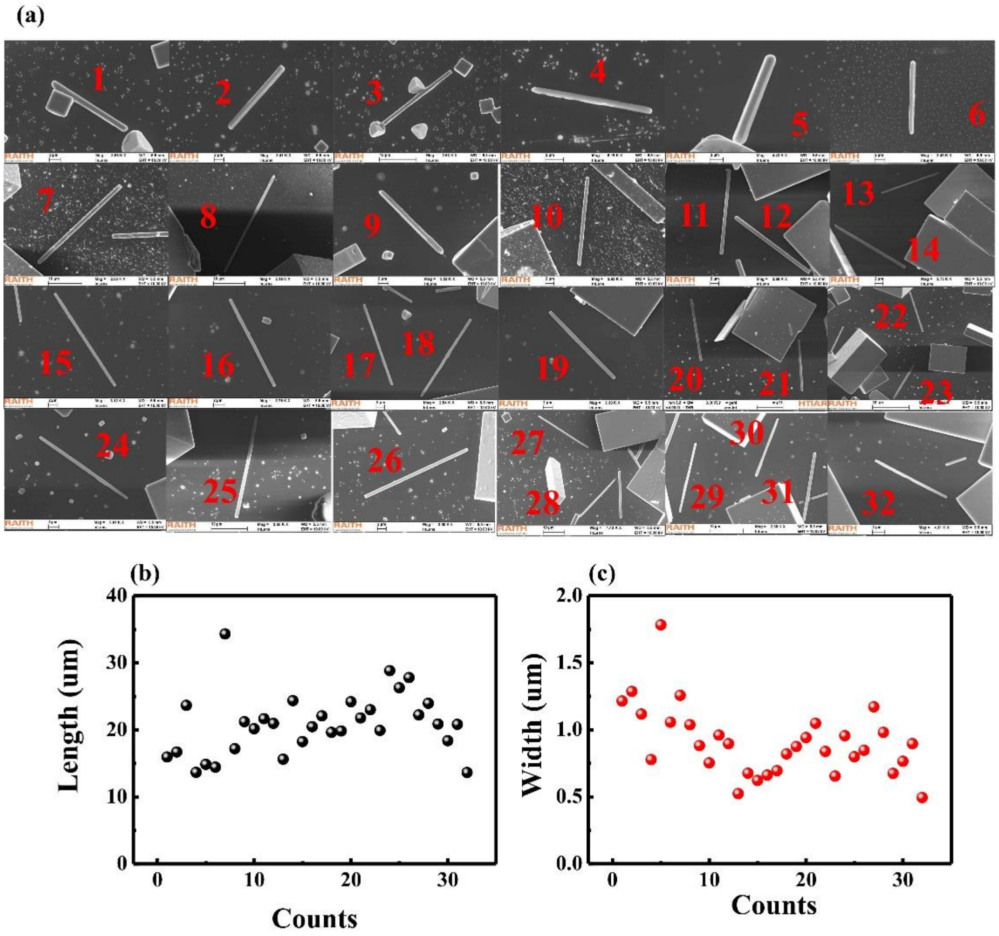


*Fig. S1: SEM images of perovskite nanowires (a) top view of the nanowires. (b) statistic length and width of the nanowires marked from 1 to 32 in (a).*

## 2. Setup for optical excitation

Here we describe the setup for optical measurement in details. An amplified ultrafast laser (1kHz, 100fs pulse width) seeded by Ti:Sapphire (Maitai, Spectraphysics) was generated and frequency doubled by a BBO crystal. Then the laser beam was coupled into a home-made fluorescent microscope (see Fig. S2(a)).  The pumping laser was focused by a 40x objective lens

into a laser spot with diameter around 75 micron. As the waveguide modes (in vertical direction) have strong diffraction in vertical direction once they leave the nanowire, the emitted light was collected by the same objective lens and all the signals were detected from the top surface. A flip mirror has been utilized to distribute emission lights into camera and spectrometer. The first one was used to take the microscope image. The latter one consisted of a spectrometer (Acton spectrapro 2700i) and a CCD camera (Princeton instrument, UV enhanced Pixis CCD). For the two-photon pumping experiment, all the set-ups are the same as single-photon excitation except that the BBO crystal was removed (see Fig. S2(b)).

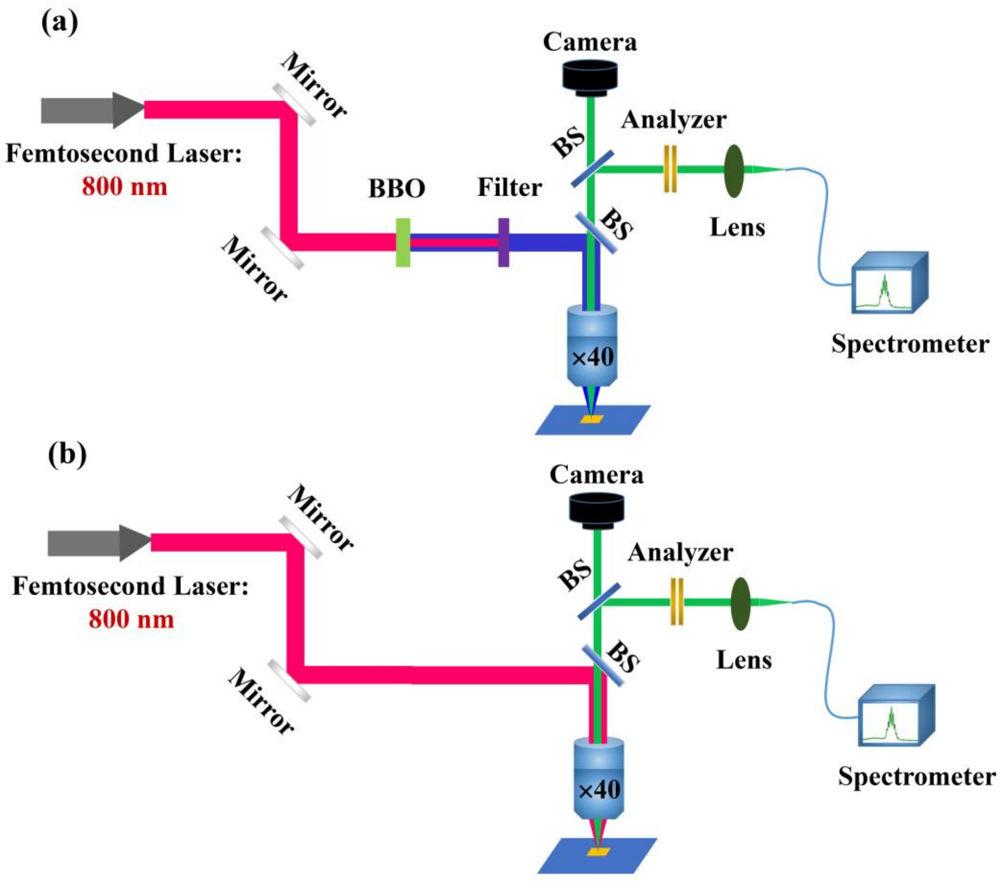


***Fig.S2****: A schematic of the home-built microscope setup for measuring the optical properties of single perovskite nanowires. (a) single-photon and (b) two-photon pumping configurations. BS: Beam Splitter*

**3. One and two-photon pumped photoluminescence**

The results in Fig. 1 of main text show the photoluminescence spectra of perovskite under single-photon pumping and two-photon pumping. Here we show more generic results of two-photon photoluminescence. As shown in Fig. S3, the photoluminescence of perovskite nanowire is a broad peak at ~ 534 nm. The full width half maximum (FWHM) is about 20 nm. Once the pumping laser was changed to 800 nm (two-photon pumping), both the width and position of the photoluminescence peak change in Fig. S3. Similar to previous reports, the emission wavelength shifted to longer wavelength and the FWHM decreased a little bit.

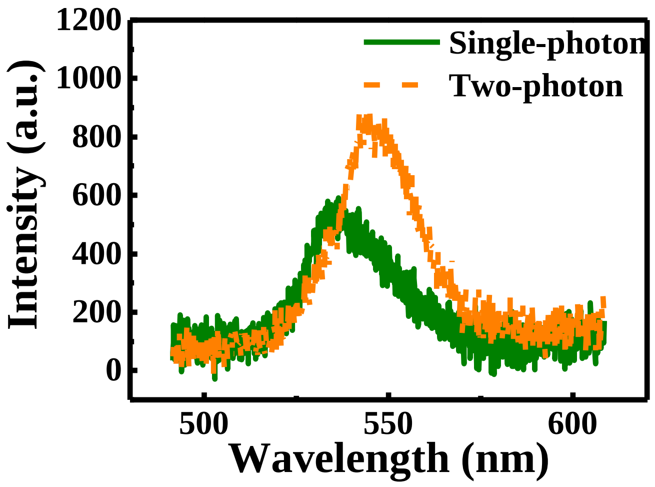


***Fig. S3***: *Photoluminescence spectra under single-photon and two-photon excitation.*

**3. Two-photon pumped lasing actions in a different perovskite nanowire**

As we mentioned in the main text, the two-photon pumped laser actions are quite generic in perovskite nanowires. Here we take nine examples to illustrate it. All the results are shown in Fig. S4. When the nanowires were excited at 927 μJ/cm$^2$, two bright spots could be clearly observed in the fluorescent microscope (see insets in Fig. S4), indicating the onsets of lasers. Meanwhile, discrete lasing peaks can be observed in all the lasing spectra.

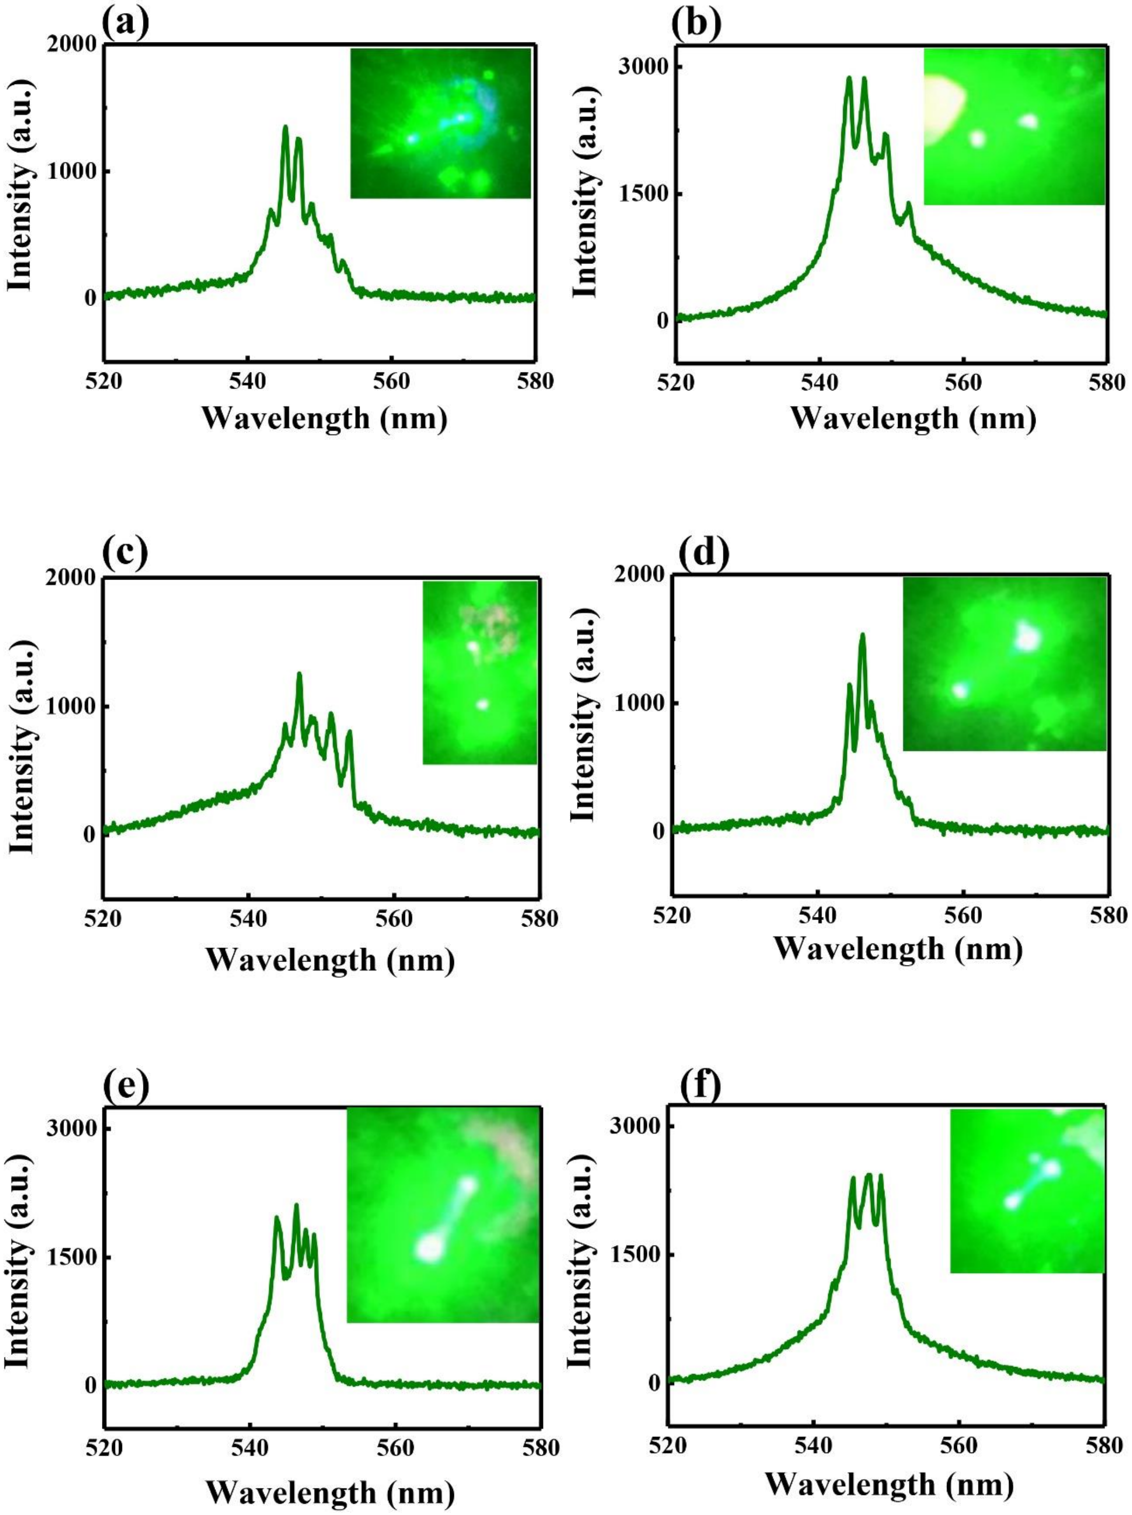
(a)
(b)
(c)
(d)
(e)
(f)
Intensity (a.u.)
Wavelength (nm)
0
1000
2000
1500
3000
520
540
560
580

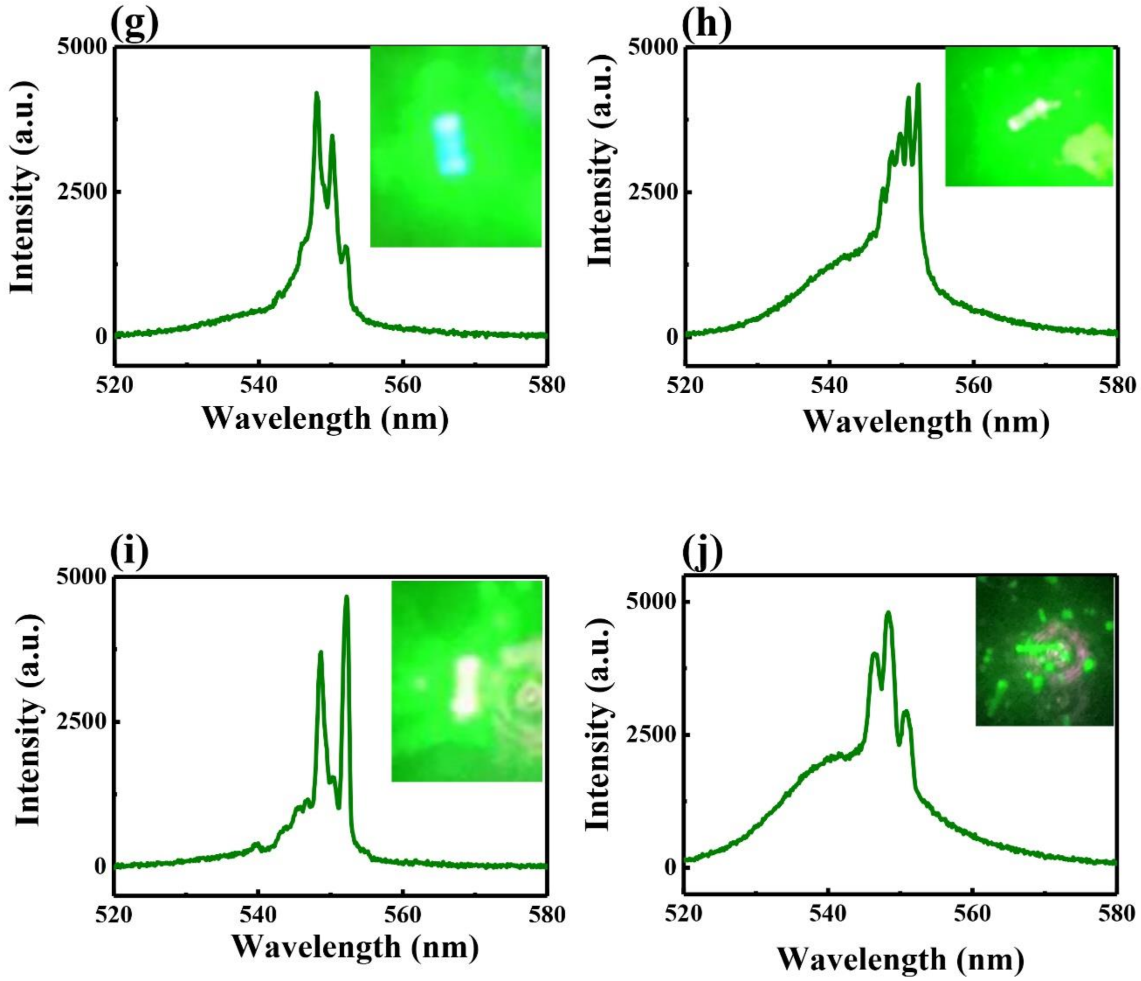


***Fig.S4***: *(a)-(j) Laser spectra of perovskite nanowires under two-photon excitation. The insets are the corresponding fluorescent microscope images.*

## 4. Numerical calculation of the mode profiles in the transverse direction

Due to the relative larger size of perovskite nanowire, the perovskite can actually support numerous of transverse waveguide modes. Here we numerically calculate the waveguide mode through mode analysis in COMSOL Multiphysics 4.3a. All the results are depicted in Fig. S5(a). We can see almost twenty waveguide modes can propagate inside the nanowire. The open squares and solid dots represent the transverse electric (TE) and transverse magnetic (TM) polarized modes, respectively. Some of their field patterns are depicted in Fig. S5(b). In Fig. 5(a),

we can see that the effective refractive index decreases at higher order waveguide modes. Interestingly, we see that their radiation losses are very close. This means that it is not very accurate to say that the fundamental modes correspond to the lasing modes because of their smaller propagating losses.

As what we have discussed in the main text, the higher order modes usually have larger incident angles on two end-facets and most of them are even totally reflected back to the nanowire. Consequently, the Q factors of higher order waveguide modes should be also higher and much easier to be excited in the lasing experiments. However, the higher order modes have much smaller effective refractive indices, which corresponding much larger mode spacings than the experimentally measure values. Considering the mode spacing, the two lowest order modes, which also have lowest Q factors, match the experimental results well. Then it is very interesting to understand this contradiction. As we mentioned in the main text, the scatters around the nanowires must be considered to solve this contradiction. Such kinds of nanosized scatters are not unique in Fig. 2 of the main text, they can also be observed in the SEM images in Fig. S1. The scatters will introduce additional scattering losses to the resonances. As the higher order modes have stronger field distributions at the boundaries, they will be significantly affected by the nanoparticles and thus be suppressed.

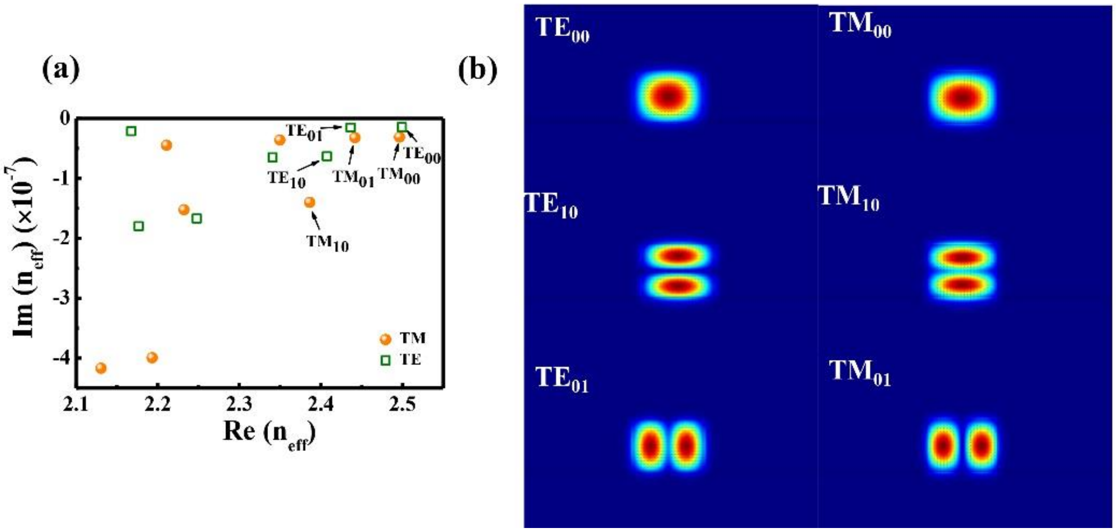


***Fig. S5***: *(a) The radiation losses of the waveguide modes in perovskite waveguide. Here the sizes of waveguide are taken from Fig. 2 in the main text. (b) The field patterns of the modes marked in a.*
